# Supplementary material for: GenBFA: An Evolutionary Optimization Approach to Bit-Flip Attacks on LLMs
Source: arXiv:2411.13757 source file (2025-07-01)
Supplement: Supplementary file 1 [file appendix.tex]

\newpage
\section{Appendix}\label{sec:appendix}

\begin{figure*}[t!]
  \centering
  \begin{subfigure}{0.32\linewidth}
    \centering
    \includegraphics[width=1.05\linewidth]
{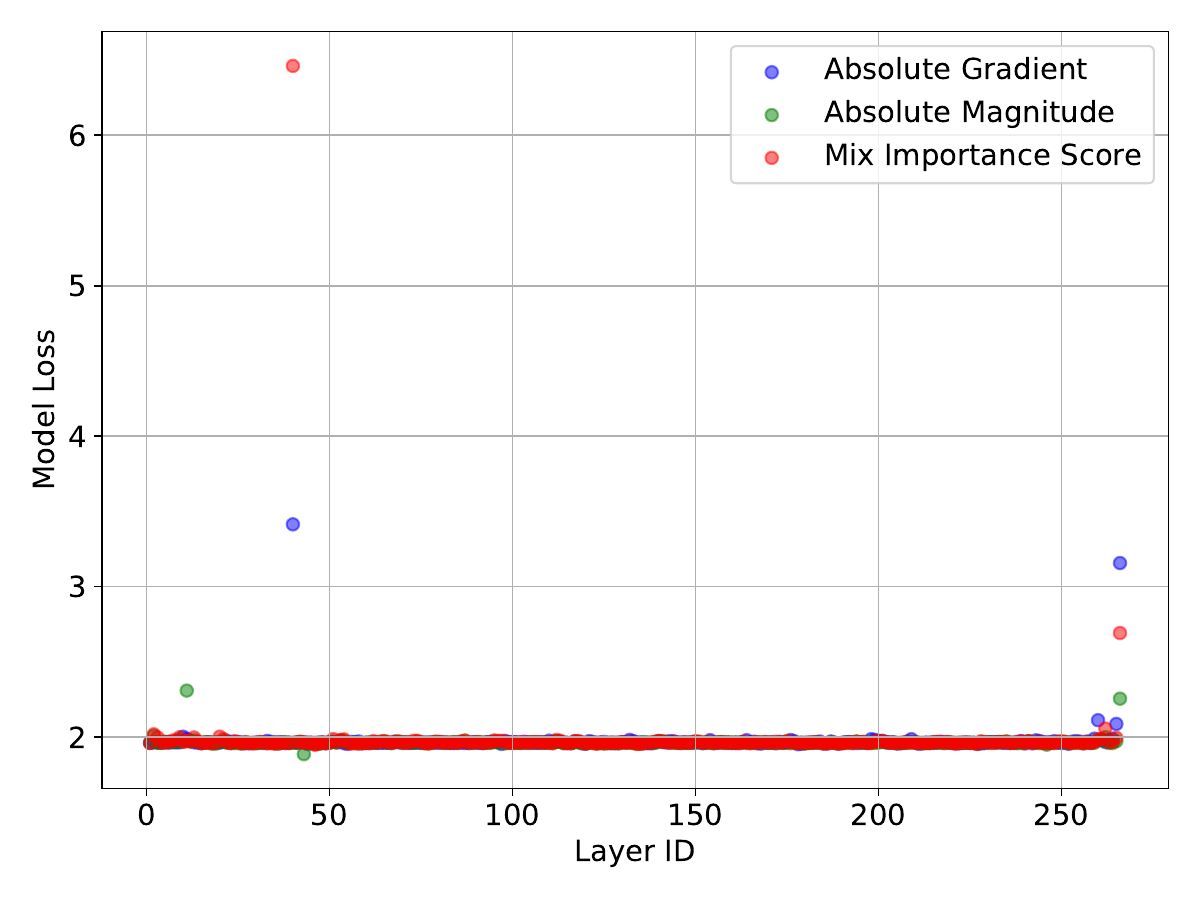}
\caption{Layer sensitivity analysis.}
  \label{fig:bitnet_layer}
  \end{subfigure}
    \hfill
  \begin{subfigure}{0.32\linewidth}
    \includegraphics[width=1.05\linewidth]
    {figures/bitnet_1.58_large_importance 1.pdf}
  \caption{Varying normalization techniques.}
  \label{fig:bitnet_weights_sensitivity}
  \end{subfigure}
  \hfill
  \begin{subfigure}{0.32\linewidth}
    \includegraphics[width=1.05\linewidth]
{figures/bitnet_1.58_large_alpha_sweep 1.pdf}
    \caption{Varying sensitivity ratio $\alpha$.}
    \label{fig:alphasweepbitnet}
  \end{subfigure}
  \caption{BitNet b1.588-bit (INT8)  experiments for (a) Layer sensitivity analysis, (b) variation of sensitivity strategies, (c) Varying sensitivity ratio $\alpha$.}
  \label{fig:BitNet1}
\end{figure*}

\begin{figure*}[t!]
  \centering
  \begin{subfigure}{0.32\linewidth}
    \includegraphics[width=1.05\linewidth]
{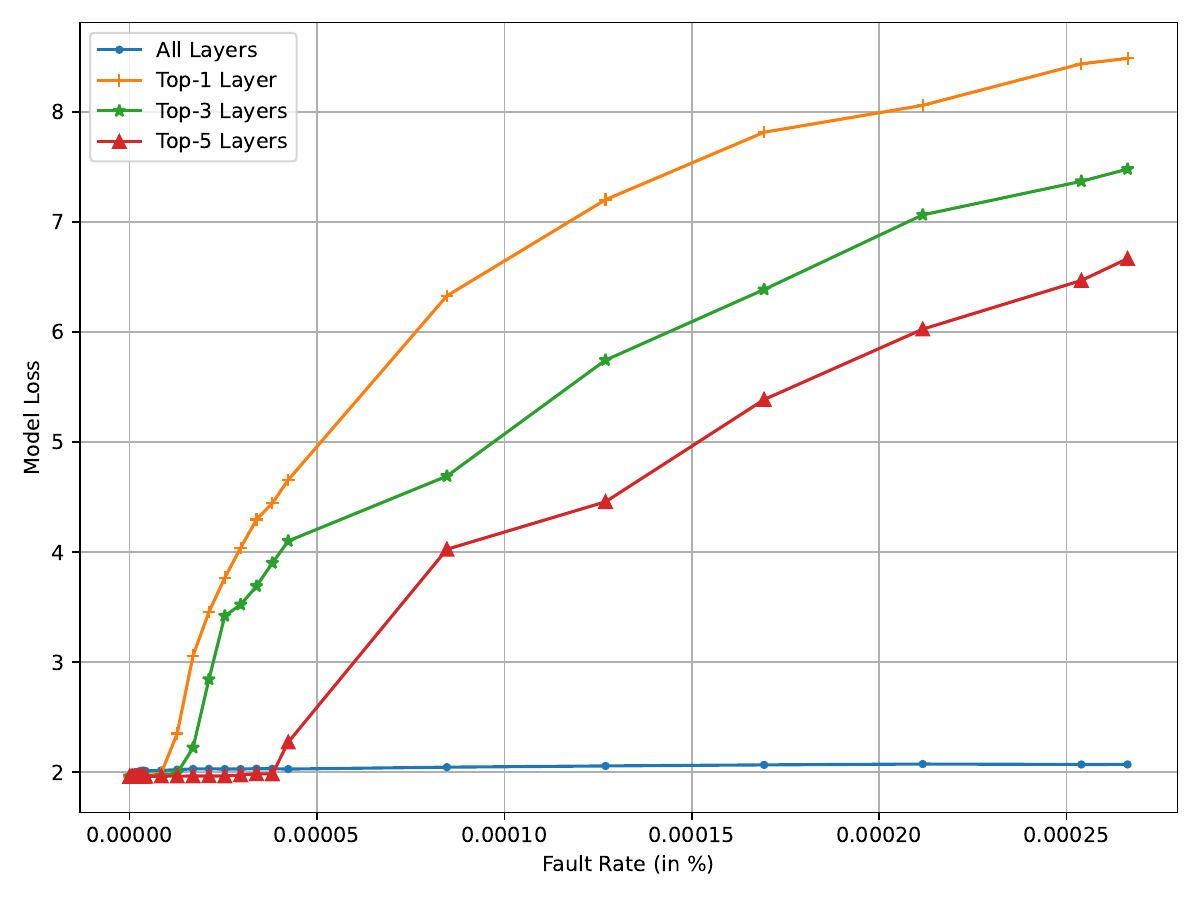}
    \caption{Varying number of layers.}
    \label{fig:layersweepbitnet}
  \end{subfigure}
  \hfill
  \begin{subfigure}{0.32\linewidth}
    \includegraphics[width=1.15\linewidth]
{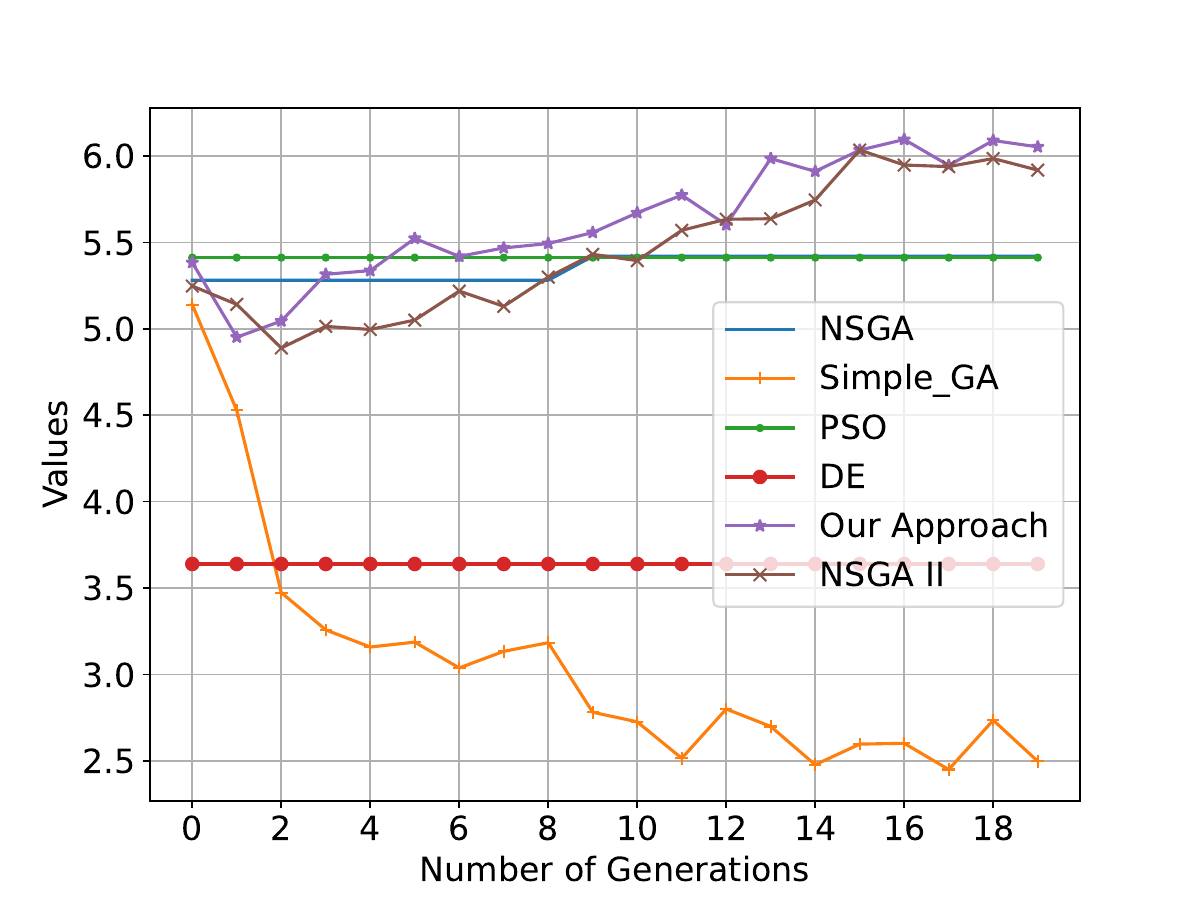}
    \caption{Varying genetic algorithms.}
    \label{fig:genetic_sweep_bitnet}
  \end{subfigure}
  \hfill
  \begin{subfigure}{0.32\linewidth}
    \includegraphics[width=1.05\linewidth]
{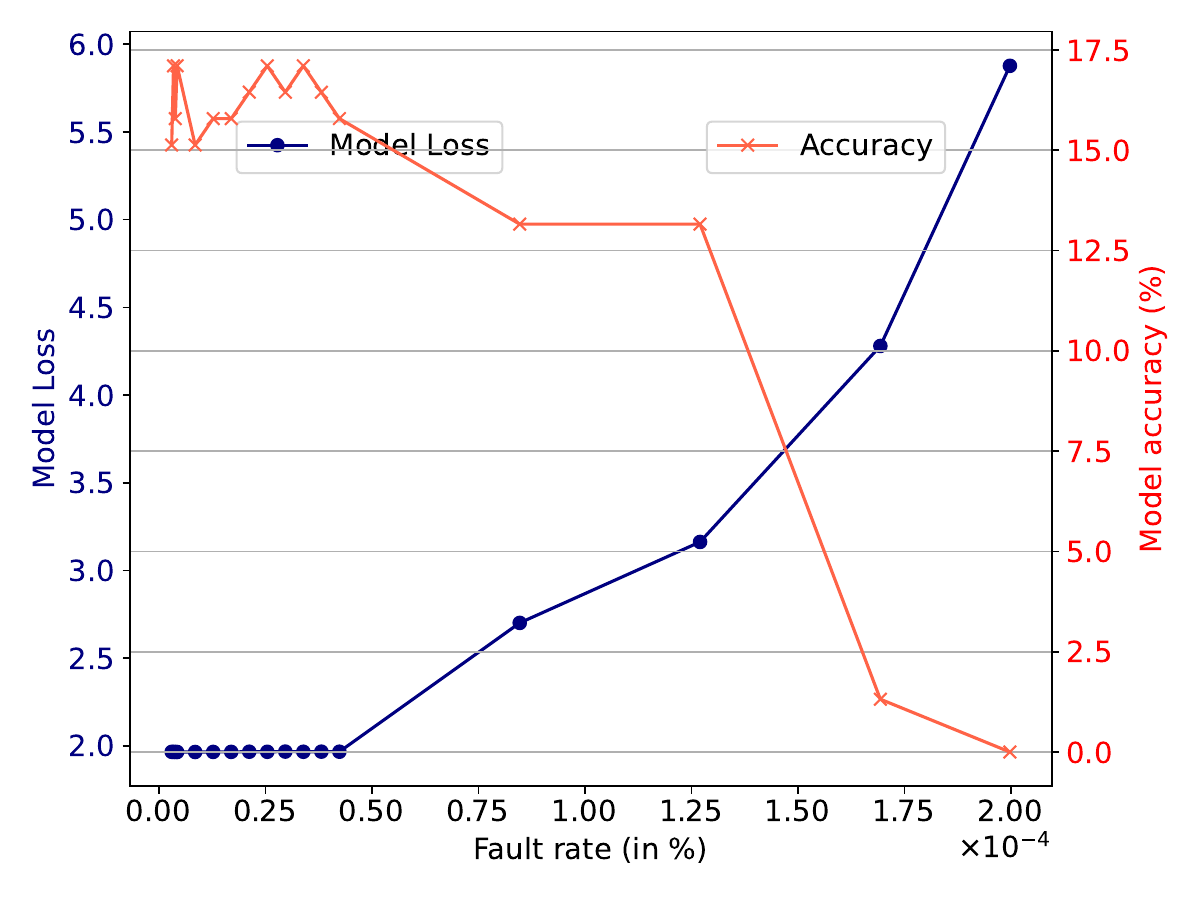}
    \caption{Weight sweep for genetic optimization.}
    \label{fig:wsweep}
  \end{subfigure}
  \caption{BitNet b1.58 8-bit (INT8) experiments for (a) varying number of layers for solution space creation, (b) varying genetic algorithms for weight subset optimization and (c) weight sweep for genetic optimization.}
  \label{fig:BitNet2}
\end{figure*}
